# Supplementary material for: Membership Privacy for Machine Learning Models Through Knowledge Transfer
Source: arXiv:1906.06589 source file (2020-12-31)
Supplement: Supplementary file 1 [file appendix_mem_worse.tex]

% !TEX root = main.tex
\section{Membership inference against highly susceptible classes}\label{appendix:worse_members}

In this section, we elaborate on the membership inference resistance that the DMP and other defenses provide to the CIFAR-10 classes with different susceptibility to membership inference. 
Specifically, we measure the membership inference resistance of different classes by plotting ROC curves, and show that the DMP trained models not only provide the on-average privacy, but also protect the classes that are highly susceptible to membership inference when no defense is used.
We perform the same measurements for DP-SGD and adversarial regularization defenses to show that, for the models with equivalent generalization error, disparity of the susceptibility to membership inference across CIFAR-10 classes is similar to our DMP defense.

\begin{figure}
\centering

\begin{tabular}{cc}
\hspace{-2em}
\subfloat{\input{new_tex_figures/cifar10_roc_baseline_redacted}
}
\hspace{-1.5em}
&
\subfloat{\input{new_tex_figures/cifar10_roc_dmp_redacted}
}

\\
\hspace{-2em}
\subfloat{\input{new_tex_figures/cifar10_roc_dp_redacted}
}
\hspace{-1.5em}
&
\subfloat{\input{new_tex_figures/cifar10_roc_advtune_redacted}
}

\end{tabular}

\caption{}

\label{fig:disparity}

\end{figure}
